# Supplementary material for: An Exposition on the Algebra and Computation of Persistent Homology
Source: arXiv:2408.07899 source file (2024-08-15)
Supplement: Supplementary file 1 [file 4B-Abelian-Category.tex]

% --------------------------
% Appendix: 
% Abelian Categories and Isomorphisms between Categories
% --------------------------

\section{Remarks on Abelian Categories and Isomorphisms on Categories}
\label{appendix:cat-abelian-theory}

Chain complexes play a huge role in this expository paper.
We gave a definition earlier for the category of chain complexes $\catchaincomplex{R}$ of $R$-modules.
In turns out that the notion of chain complex can be generalized to arbitrary categories that have certain properties, 
i.e.\ a chain module $(C_n, d_n)_{n \in \ints}$ need not be $R$-modules.
This section provides a brief discussion of \textbf{abelian categories}, which are categories that allow this chain complex construction.

Note that this will not be a rigorous discussion on abelian categories 
and what we will present are often simplified versions of definitions, 
	versions that we have determined to be acceptable enough to provide motivation for the results presented regarding persistence modules.
	The background needed in order to rigorously define abelian categories are massively out of scope of this paper.
For a more detailed and careful treatment of this topic, we recommend the paper \textit{Abelian Categories and Mitchell's Embedding Theorem} by James Bailie~\cite{cattheory:bailie}.

In a roundabout approach, we first give a characterization of abelian categories taken from~\cite[Section E.5]{cattheory:rhiel} and define the required constructions after this definition.

\begin{definition}
	A category $\catname{A}$ is an \textbf{abelian category} if 
	\begin{enumerate}
		\item $\catname{A}$ has a {zero object} $0_\catname{A}$.
		\item For all objects $X$ and $Y$ in $\catname{A}$, the {direct sum} $X \oplus Y$ exists.
		\item Kernels and cokernels of all morphisms in $\catname{A}$ exist.
	\end{enumerate}
\end{definition}
\begin{miniremark}
	This is technically a characterization of abelian categories. Rhiel states this in~[page 139]\cite{cattheory:rhiel} as a consequence of Freyd-Mitchell's Embedding Theorem~\cite[Theorem E.5.2]{cattheory:rhiel}.
	% which roughly states that abelian categories is a (full) subcategory of the category $\catmod{R}$ for some ring $R$. In other words, we can generally assume that objects and morphisms in an abelian category act the same way as $R$-modules and $R$-module homomorphisms.
\end{miniremark}

Below, we present characterizations of the zero morphism, direct sum, kernel, and cokernel in terms of universal properties. 
Note that the terms here are restricted to the case of abelian categories.
For example, the direct sum construction in abelian categories is only called a direct sum when two constructions called the product and coproduct yield the same object. 
The following definitions are adapted from 
\cite[Section 2.3]{persmod:bubenik-categorification},
\cite[Section 3.1]{cattheory:rhiel}
and~\cite{cattheory:bailie}.

\begin{definition}
	The following constructions are defined by \textbf{universal properties}, which are diagrams that require the existence and uniqueness of certain morphisms.
	Let $\catname{A}$ be some category.
	\begin{enumerate}
		\item 
		A \textbf{zero object} $0_\catname{A}$
			in $\catname{A}$ is an object such that for every object $X$ in $\catname{A}$, there is exactly one morphism $0_\catname{A} \to X$ and exactly one morphism $X \to \catname{A}$.
			The universal property $0_\catname{A}$ must satisfy is as follows:
			\begin{center}
				\includegraphics[width=0.4\linewidth]{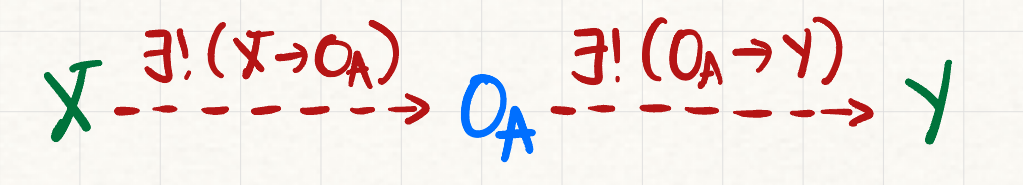}
			\end{center}
			For all items below, assume that $0_\catname{A}$ exists. 

			The existence of zero objects imply the existence of {zero morphisms}. 
			Given objects $X$ and $Y$ in $\catname{A}$, the \textbf{zero morphism} $0_{X,Y}: X \to Y$ is defined by the composition $0_{X,Y}: X \to 0_\catname{A} \to Y$. Note that the composition is unambiguous by uniqueness of the morphisms related to $0_\catname{A}$.

		\item 
			A \textbf{direct sum} $X \oplus Y$ of objects $X \oplus Y$ in $\catname{A}$ is an object in $\catname{A}$ along with morphisms $\pi_X: X \oplus Y \to X$ and $\pi_Y: X \oplus Y \to Y$ called \textbf{projection morphisms} such that 
			given any pair of morphisms $f_X: A \to X$ and $f_Y: A \to Y$ for any object $A$, there exists a unique morphism $f: A \to X \oplus Y$, as illustrated below:
			\begin{center}
				\includegraphics[width=0.35\linewidth]{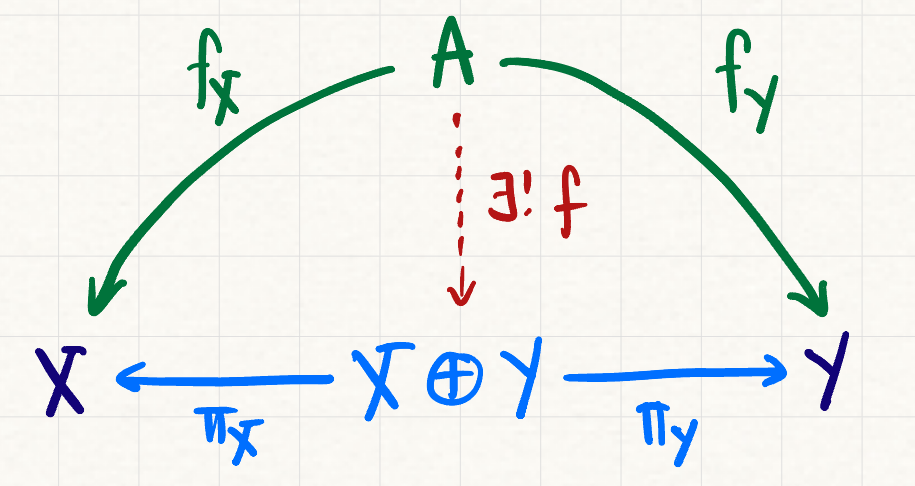}
			\end{center}
			When direct sums are defined, the construction is commutative and associative up to isomorphism.

		\item 
			The \textbf{kernel} $\ker(f) = (K,k)$ of a morphism $f: X \to Y$ in $\catname{A}$ is a tuple of an object $K$ and a morphism $k: K \to X$
			such that given any morphism $g: W \to X$ such that $f \circ g = 0_{W,Y}$, there exists a unique morphism $\bar{g}: W \to K$ such that $k \circ \bar{g} = g$, as illustrated below:
			\begin{center}
				\includegraphics[width=0.25\linewidth]{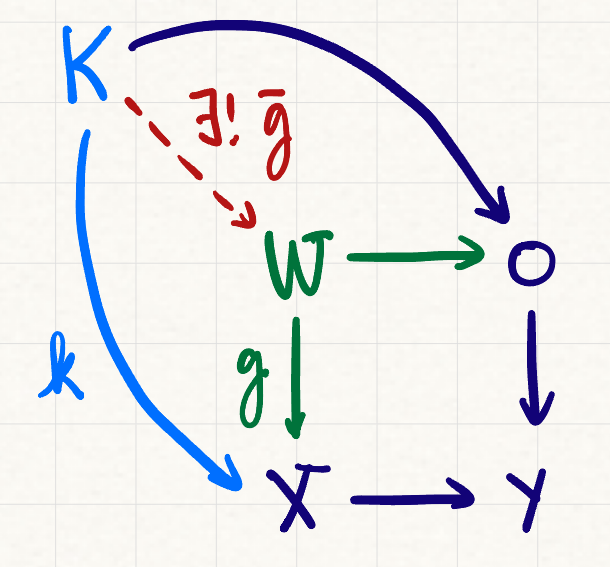}
			\end{center}

		\item 
			The \textbf{cokernel} $\coker(f) = (Q,q)$ of a morphism $f: X \to Y$ in $\catname{A}$ is a tuple of an object $Q$ and a morphism $q: Y \to Q$ such that given any morphism $h: Y \to Z$ such that $h \circ f = 0_{X,Z}$, there exists a unique morphism $\bar{h}: Q \to Z$ such that $\bar{h} \circ q = h$, as illustrated below:
			\begin{center}
				\includegraphics[width=0.25\linewidth]{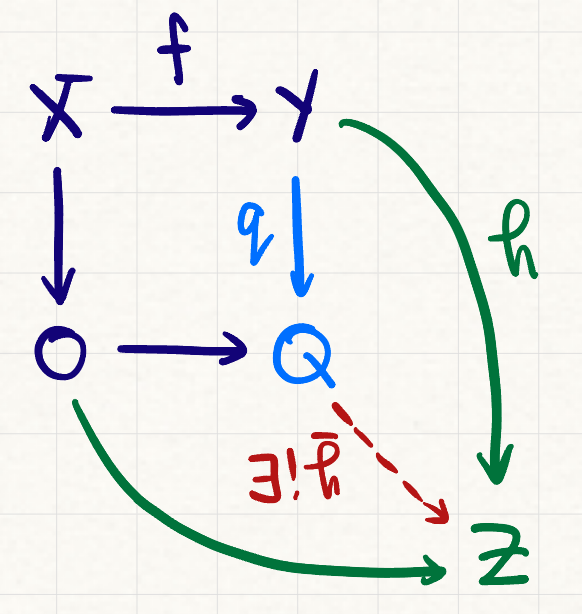}
			\end{center}
	\end{enumerate}
	When these objects are defined, they are unique up to (unique isomorphism).
\end{definition}
\noindent Some key remarks:
\begin{enumerate}
	\item 
	One key observation here is that the notions of direct sums, kernels, and cokernels for any abelian category must match the definition given above.
	This will be relevant once we use an isomorphism between categories.

	\item 
	For this expository paper, we will define the notions of zero objects, direct sums, kernels, and cokernels concretely. We would only need to define these for the category of persistence modules 
	but we include this here for the category isomorphism to make sense.

	\item 
	Most of the categories we will work with such as $\catvectspace$, $\catmod{R}$ and $\catgradedmod{R}$ are all abelian categories.

	\item 
	Observe that kernels and cokernels are defined to be a pair of an object and a morphism. 
	However, since kernels uniquely determine both, some abuse of notation is done and we use the term kernel and cokernel to refer to the object instead, i.e.\ write $\ker(f) = K$ and $\coker(f) = Q$, as denoted above.

	In categories like $\catvectspace$, $\catmod{R}$ and $\catgradedmod{R}$ (i.e.\ most of the categories we encounter before studying category theory), the morphisms of the kernel and cokernel are usually uninteresting. For example, the morphism $k: K \to X$ of the kernel $\ker(f) = (K, k)$ is usually the injection map.

	\item 
	The last line on the definition says something about unique isomorphism. We have not defined \textit{unique} isomorphisms in this paper. However, roughly speaking, this means that the object assignment of direct sum, kernel, and cokernel construction is unambiguous, e.g.\ the direct sum $X \oplus Y$ does not yield two different objects.

	\item 
	The constructions for \textbf{subobject} and \textbf{image} can be characterized by the kernel and cokernel of certain morphisms. 
	Since we mainly talk about abelian categories as motivation for an approach via category theory, it suffices to state that subobjects and images are also determined by universal properties and will transfer through category isomorphism (defined below).
\end{enumerate}

\noindent 
As mentioned earlier, we can create chain complexes for abelian categories. 
The definitions are similar to that of $\catchaincomplex{R}$ but we state it here for completion.

\begin{definition}\label{defn:chain-complex-on-abelian-cats}
	Let $\catname{A}$ be an abelian category.
	\begin{enumerate}
		\item A \textbf{chain complex} on $\catname{A}$ is a collection $A_\bullet = (A_n, \alpha_n)_{n \in \ints}$ of objects $A_n$ and morphisms $\alpha_n: A_n \to A_{n-1}$ such that for all $n \in \ints$, $\alpha_{n+1} \circ \alpha_n = 0$ (the zero morphism).
		\item The \textbf{$n$\th chain homology} $H_n(A_\bullet)$ of a chain complex $A_\bullet$ is given by 
		\begin{equation*}
			H_n(A_\bullet) = \ker(\alpha_n) \,/\, \image(\alpha_{n+1})
		\end{equation*}
	\end{enumerate}
\end{definition}
\noindent\textit{Remark: }
We do want to state that what is given above is not the conventional way to state the generalization of chain complexes to abelian categories.
We believe a key justification of this involves Freyd-Mitchell's Embedding Theorem~\cite[Theorem E.5.2]{cattheory:rhiel}.
This theorem roughly states that that abelian category $\catname{A}$ is a (full) subcategory of some category $\catmod{K}$ for given ring $K$. 
As such, we can essentially do the chain complexes of $\catname{A}$ in the category of $\catmod{K}$, the category of $K$-modules.

\noindent 
In persistence theory, we are also interested in a notion of equality or similarity of categories. 
Under certain conditions, a strong notion of equality between abelian categories will allow us to get a correspondence between the notions of direct sums, kernels, cokernels, and images for the two categories.
We provide a definition of this below taken from~\cite[Definition 1.1.9]{cattheory:rhiel}

\begin{definition}\label{defn:cats-isom}
	An \textbf{isomorphism of categories} between categories $\catname{C}$ and $\catname{D}$ is given by a pair of functors $F: \catname{C} \to \catname{D}$ and $G: \catname{D} \to \catname{C}$ such that
	\begin{equation*}
		\begin{aligned}
			(G \circ F)(C) &= C &\text{ for all objects } C \text{ in } \catname{C} 
			\\
			(G \circ F)(\alpha) &= \alpha &\text{ for all morphisms } \alpha \text{ in } \catname{C} 
		\end{aligned}
		\qquad\text{ and }\qquad 
		\begin{aligned}
			(F \circ G)(D) &= D &\text{ for all objects } D \text{ in } \catname{D} \\
			(F \circ G)(\delta) &= \delta &\text{ for all morphisms } \delta \text{ in } \catname{D}
		\end{aligned}
	\end{equation*}
	Equivalently, $F$ and $G$ represent a category isomorphism if $F \circ G = \id_\catname{D}$ and $G \circ F = \id_\catname{C}$ with $\id_\catname{C}$ and $\id_\catname{D}$ denote the identity functor on $\catname{C}$ and $\catname{D}$ respectively.
\end{definition}

\noindent 
If we can provide functors $F$ and $G$ as above between two abelian categories, the constructions like those described above can essentially be treated as commutative with respect to the functors $F$ and $G$.
We provide a characterization of this below, taken from~\cite[Theorem 27]{cattheory:bailie}.

\begin{proposition}
	Let $\catname{A}$ and $\catname{X}$ be abelian categories and let $F_X: \catname{A} \to \catname{X}$ and $F_A: \catname{X} \to \catname{A}$ represent an isomorphism of categories. Then, $F_X$ and $F_Y$ preserve the following:
	\vspace{0.5\baselineskip}
	\begin{multicols}{4}
		\begin{enumerate}
			\item finite direct sums 
			\item zero object 
			\item kernels
			\item cokernels 
			\item images
			\item exact sequences
			\item chain homology
		\end{enumerate}
	\end{multicols}
\end{proposition}

%-------------------
