# Supplementary material for: An Exposition on the Algebra and Computation of Persistent Homology
Source: arXiv:2408.07899 source file (2024-08-15)
Supplement: Supplementary file 2 [file 0-appendix.tex]

% !TEX root = 0-appendix.tex
\documentclass[class=report, crop=false]{standalone}
\usepackage{../A2-customcommands}
\addbibresource{../A2-References.bib} 

\usepackage{xr}
	\externaldocument{../B1A-Homology/aux/0-b1a-homology}
	\externaldocument{../B2-Persistence/aux/0-b2-persistence}
	\externaldocument{../B3-Persistent-Homology/aux/0-b3-persistent-homology}
	\externaldocument{../B4-Matrices/aux/0-matrix-calculation}
	%\externaldocument{../C1-Appendix/aux/0-appendix}
\graphicspath{{../images/}}

\DRAFTMODE

\begin{document} 
	\onlyifstandalone{
		\renewcommand*\contentsname{Table of Contents}
		\pdfbookmark{\contentsname}{toc}
		\begin{spacing}{1.2} 
			\tableofcontents 
		\end{spacing} 
		\clearpage
	}

	\appendix
	\titleformat{\section}[hang]{\large\bfseries}{Appendix \thesection.}{1em}{}[\vspace{-10pt}\grayline] 
	\renewcommand{\thesection}{A\arabic{section}}%
	%\chapter*{Appendices}% 
	\addcontentsline{toc}{chapter}{Appendices}
	%https://tex.stackexchange.com/questions/4102/setting-setcountertocdepth-for-an-individual-chapter
		\input{"1-Miscellaneous.tex"}\clearpage
		\input{"3A-Matrix-Theory.tex"}\clearpage
		\input{"3B-Module-Theory.tex"}\clearpage
		\input{"4A-Category-Theory.tex"}

\end{document}
